# Supplementary material for: Assuming Just Enough Fairness to make Session Types Complete for Lock-freedom
Source: arXiv:2104.14226 source file (2021-04-29)
Supplement: Supplementary file 1 [file appendix.tex]

% !TEX root = main.tex
\comP[H]{the following has not been split into separate appendices}
This appendix contains proofs of theorems in body of paper and extended classifications

<<<<<<< HEAD
\subsection{Soundness proofs}

\comH{Warning: In a state of transformation.}

\newcommand{\residual}[2]{{ _{#1}\!\!\setminus\!\! \left( {#2} \right) }}

\begin{lemma}{guarded1}
Projection type $\rec{X} \PP$ is guarded iff $\PP\sub{X}{\rec{X} \PP}$ is guarded.
\end{lemma}

\begin{lemma}{guarded2}
We have $\proj{p}{\rec{X} \G} = \rec{X}\PQ$ iff $\proj{p}{\G\sub{X}{\rec{X} \G}} = \PQ\sub{X}{\rec{X}\PQ}$.
\end{lemma}

The following is required since we require also that the labels are equal to for a race between two parties in the reactive semantics $\dgoesto{}$, which is not required for $\goesto{}$, since the internal choice will select exactly one label in such scenarios.  
Also, $\proc(p, \N')$ and $\proc(p, \N'')$ may be different, since there may be two different internal choices made by $p$ that commit to two different continuations for $p$, before the communication occurs, according to $\goesto{}$.  
\begin{lemma}{race}
If a network $\N$ is race free and $\N \dgoesto{\comm{p}{\lambda}{r}~} \N'$ and $\N \dgoesto{\comm{q}{\mu}{r}~} \N''$,
then $p = q$ and if $\lambda = \mu$ then $\proc(r, \N') = \proc(r, \N'')$.
\end{lemma}

\begin{definition}{global transition}
If $\G$ is a global type
and $\comm{p}{\lambda}{q}$ is a transition.
We $\G'$ define as $\residual{\comm{p}{\lambda}{q}}{\G}$
according to the following transformation on global types. 
\[
 \residual{\comm{p}{\lambda}{q}}{\rec X\GH} =
\residual{\comm{p}{\lambda}{q}}{\GH \sub{X}{\rec X\GH} } 
\]
\[
\begin{array}{l}
 \residual{\comm{p}{\lambda}{q}}{
    \bigboxplus_{k \in K}
    \comm{r}{\lambda_k}{s_k};\GH_k
 }
\\\qquad
 = 
\left\{
\begin{array}{l}
\GH_k \quad \mbox{if $r = p$ and $\lambda_k = \lambda$ and $s_k = q$}
\\
    \bigboxplus_{k \in K}
    \comm{r}{\lambda_k}{s_k};
 \residual{\comm{p}{\lambda}{q}}{
  \GH_k
 }
\quad \mbox{otherwise}
\end{array}
\right.
\end{array}
\]
We say that $\G \goesto{\comm{p}{\lambda}{q}} \G'$.
\end{definition}
The relation $\G \goesto{\comm{p}{\lambda}{q}} \G'$ is well-defined for the relevant situations where $\N \vdashg \G$, $\N$ is race-free and $\N \dgoesto{\comm{p}{\lambda}{q}} \N'$.

Lemma~\ref{lem:subject reduction} follows immediately from the following stronger session fidelity result.

\begin{lemma}{session fidelity}
For race-free networks $\N$, if and $\N\dgoesto{\alpha}\N'$
and $\N \vdashg \G$, then there exists $\G'$ such that
$\G \goesto{\alpha} \G'$ and $\N' \vdashg \G'$.
\end{lemma}

\begin{proof}
Assume that $\N \vdashg \G$ holds and suppose we have a transition $\N \dgoesto{\comm{p}{\lambda}{q}} \N'$.

Firstly, observe that, by unfolding the rules for transitions we have.
\commH{Common with Rob's claim 1.}
\begin{itemize}
\item $\proc(p, \N) = \rec{X_1} \ldots \rec{X_m} \bigoplus_{i\in I} \send{q_i}{\lambda_i}\PP_i$,
where $q = q_i$ and $\lambda= \lambda_i$ for some $i\in I$,
\item  
$\proc(q, \N) = \rec{Y_1} \ldots \rec{Y_n} \sum_{j\in J} \recv{p_j}{\lambda_j}\PQ_i$,
where $p = p_j$ and $\lambda = \lambda_j$ for some $j \in J$.
\end{itemize}
Furthermore, we have
$\proc(p, \N') = \PP'_i$, where $\PP'_i$ is the unfolding of $\PP_i$ according the fixed points,
$\proc(q, \N') = \PQ'_j$, where $\PQ'_j$ is the unfolding of $\PQ_j$ according the fixed points,
and $\proc(r, \N') = \proc(r, \N)$ otherwise.

The rest of this proof establishes $\G'$ such that $\G \goesto{\comm{p}{\lambda}{q}} \G'$ is well-defined 
and 
that $\N' \vdashg \residual{\comm{p}{\lambda}{q}}{\G}$.
The proof proceeds by by induction, where the induction measure is the maximum depth of a choice with a branch where $\comm{p}{\lambda}{q}$ occurs in the tree of choices in $\G$.\commH{Common with Lemma 6.}
Note this distance is always finite due to the fact that $\proj{p}{\G}$ and $\proj{q}{\G}$ are guarded.

\textbf{Base case.}
Consider when $\G$ is of the following form.
\[
\rec{Z_1} \ldots \rec{Z_\ell} \boxplus_{k\in K} \send{p}{\lambda_k}{s_k}\GH_k
\]
%The unfolding of $\G$ is $\G' = \boxplus_{k\in K} \send{p}{\lambda_k}{s_k}\GH'_k$, such that $\N \vdashg \G'$.
In this case, it is immediate that we have for following projection of $p$, which is a guarded projection type.
\[
\proj{p}{\G} = \rec{Z_1} \ldots \rec{Z_\ell} \bigoplus_{i\in K} \send{s_i}{\lambda_i}\proj{p}{\GH_i}
\]
Hence, by the type rule for recursion and $\bigoplus$, since $\rec{X_1} \ldots \rec{X_m} \bigoplus_{i\in I} \send{q_i}{\lambda_i}\PP_i \vdashg \proj{p}{\G}$,
 we have $I \subseteq K$ and for all $i \in I$, we have $\PP'_i \vdash \proj{p}{\GH'_i}$, where $\PP'_i$ and $\GH'_i$ are the unfoldings of $\PP_i$ and $\GH_j$ with the respective recursive calls.
Indeed, we have $\PP'_i \vdashg \proj{p}{\GH'_i}$ since unfolding preserves guardedness.
%Observe here, that it must be the case that for some $i \in K$, we have $s_i = q$ and $\lambda_i = \lambda$, otherwise there would be no transition $\proj{p}{\G} = \rec{Z_1} \ldots \rec{Z_\ell} \bigoplus_{i\in K} \send{s_i}{\lambda_i}\proj{p}{\GH_i}
Therefore, from the analysis of the transition rules above, for some $i \in I$, we have  $\lambda = \lambda_i$ and $q = q_i$,
and hence since $I \subseteq K$, we have for some $i \in K$ we have  $\lambda = \lambda_i$ and $q = q_i$.\footnote{This idea at this point is that, along every path of the global type, the first choice involving $p$ as a sender must include the option of sending $\lambda$ to $q$, otherwise there would be some other output from $p$ before hand preventing the transition.}

Now consider the following projection.
\[
\proj{q}{\G} = \rec{Z_1} \ldots \rec{Z_\ell} \merge_{k\in K} \proj{q}{\comm{p}{\lambda_k}{s_k} ; \GH_k}
\]
So, we have the following.
\[
\rec{Y_1} \ldots \rec{Y_n} \sum{j\in J} \recv{p_j}{\lambda_j}\PQ_i \vdashg \merge_{k\in M} \proj{q}{\comm{p}{\lambda_k}{s_k} ; \GH_k}
\]
Therefore, by the type rule for merge and fixed points,
we have for all $k \in M$, that $\sum{j\in J} \recv{p_j}{\lambda_j}\PQ'_j \vdash \proj{q}{\comm{p}{\lambda_k}{s_k} ; \GH'_k}$,
where $\PQ'_j$ and $\GH'_k$ are obtained by unfolding $\PQ_j$ and $\GH_k$ respectively.
Now, recall that for some $i \in K$ we have $\lambda_i = \lambda$ and $s_i = q$;
hence we have $\proj{q}{\comm{p}{\lambda_i}{s_i} ; \GH'_i} = \recv{\lambda}{p}; \proj{q}{ \GH'_i }$.
Therefore, by the type rule for $\sum$ it must be that for for some $j' \in J$ (where $j'$ is not necessarily $j$ defined above) we have $p_{j'} = p$ and $\lambda_{j'} = \lambda$,
and
$\PQ'_{j'} \vdash \proj{q}{ \GH'_i }$, indeed, since unfolding preserves guardedness, we have $\PQ'_{j'} \vdashg \proj{q}{ \GH'_i }$.
Now we appeal to race-freedom, and the fact that, by the rules for transitions $\N \dgoesto{\comm{p}{\lambda}{q}} \N''$, 
where $\proc(q, \N'') = \PQ'_{j'}$.
By Lemma~\ref{lem:race}, since we began by assuming that $\N \dgoesto{\comm{p}{\lambda}{q}} \N'$, and $\N$ is race-free it must be the case that $\N'$ = $\N''$ and hence $\PQ'_{j'} = \proc(q, \N'') = \proc(q, \N') = \PQ'_{j}$.
\footnote{When seeking condition for soundness that is necessary (race-freedom is only a sufficient condition), we need not have that $\PQ'_{j'} = \PQ'_{j}$, but we would require only that if there is such a race then both resulting networks inhabit the type $\proj{q}{ \GH'_i }$.}

We conclude this case by observing that for $r \neq p$ and $r \neq q$, we have
\[
\proj{r}{\GH} = \rec{Z_1} \ldots \rec{Z_\ell} \merge_{k\in K} \proj{r}{\comm{p}{\lambda_k}{s_k} ; \GH_k}
\]
Hence, by the type rules for fixedpoints and merge, 
we have for all $k \in K$, that $\proc(r, \N') \vdashg \proj{r}{\comm{p}{\lambda_k}{s_k} ; \GH'_k}$.
Thus, since $p \neq r$ and $s_i = q$ and $q \neq r$, for $i \in K$, we have $\proc(r, \N') \vdashg \proj{r}{\GH'_i}$.

Thereby we have $\N' \vdashg \GH'_i$, and furthermore we have $\residual{\comm{p}{\lambda}{q}}{\G} = \GH'_i$, as required.

\textbf{Inductive case.}
Now consider the inductive case, where $\G$ is of the form below where $r \neq p$.
\[
\rec{Z_1} \ldots \rec{Z_\ell} \boxplus_{k\in K} \comm{r}{\mu_k}{s_k}\GH_k
\]
Observe that for all $k \in K$ we also have $s_k \neq p$, otherwise the first actions in $\proc(p, \N)$ would be a number of fixedpoint operator followed by an external choice.
Hence we have $\proj{p}{\G} = \rec{Z_1} \ldots \rec{Z_\ell} \merge_{k\in K} \proj{p}{\GH_k}$.
Since $\rec{X_1} \ldots \rec{X_m} \bigoplus_{i\in I} \send{q_i}{\lambda_i}\PP_i \vdashg \rec{Z_1} \ldots \rec{Z_\ell} \merge_{k\in K} \proj{p}{\GH_k}$,
by the rules for fixedpoints and merge, for all $k \in K$, we have 
$\bigoplus_{i\in I} \send{q_i}{\lambda_i}\PP'_i \vdash \proj{p}{\GH'_k}$, where $\GH'_k$ is the unfolding of $\GH_k$ w.r.t., the fixedpoints indicated.
Similarly, we have $\proj{q}{\G} = \rec{Z_1} \ldots \rec{Z_\ell} \merge_{k\in K} \proj{q}{\GH_k}$, so, for each $k\in K$, we have $\sum_{j\in J} \recv{p_j}{\lambda_j}\PQ'_i \vdash \proj{q}{\GH_k}$.

Now, consider all $k \in K'$ where $K'$ is a maximal subset of $K$ such that $\N \dgoesto{\comm{r}{\mu_k}{s_k}} \N_k$ and $\N_k \vdashg \GH_k$.
Clearly, $\N_k \dgoesto{\comm{p}{\lambda_i}{s_i}} \N'_k$, since the transition involving $r$ and $s_k$ cannot interfere with $p$ or $q$.
Also, the induction measure, described above, decreases in $\GH_k$ compared to $\G$.
Thus we can apply the induction hypothesis, to obtain that $\N'_k \vdashg \residual{\comm{p}{\lambda}{q}}{\GH_k}$.

We now aim for show that $\N' \vdashg  \residual{\comm{p}{\lambda}{q}}{\G}$.
We make the following observations.
\begin{itemize}
\item We have, for all $k\in K'$, that $\proc(p, \N') = \proc(p, \N'_k )$,
also we have seen that $\proc(p, \N'_k ) \vdashg \residual{\comm{p}{\lambda}{q}}{\GH_k}$.
Hence, by the type rule for merge, we have the following.
\[
\proc(p, \N') \vdashg \merge_{i \in K'} \residual{\comm{p}{\lambda}{q}}{\GH_k}
\]
Observe that the above is equivalent to $\proc(p, \N') \vdashg \residual{\comm{p}{\lambda}{q}}{ \boxplus_{k \in K'} \comm{r}{\mu_k}{s_k}; \GH_k}$.

\item We have, for all $k\in K'$, that $\proc(q, \N') = \proc(q, \N'_k )$,
also we have seen that $\proc(q, \N'_k ) \vdashg \residual{\comm{p}{\lambda}{q}}{\GH_k}$.
Hence, by the type rule for merge, we have the following.
\[
\proc(q, \N') \vdashg \merge_{i \in K'} \residual{\comm{p}{\lambda}{q}}{\GH_k}
\]
Observe that the above is $\proc(q, \N') \vdashg \residual{\comm{p}{\lambda}{q}}{ \boxplus_{k \in K'} \comm{r}{\mu_k}{s_k}; \GH_k}$.

\item If $s \neq p$ and $s \neq q$, then $\proc(s, \N') = \proc(s, \N)$
also $\proc(s, \N) \vdashg \proj{s}{\G}$; hence, by \textit{Observation 2} below, $\proc(s, \N') \leq_g \residual{\comm{p}{\lambda}{q}}{ \proj{s}{\G} }$.

\textit{Observation 2.}
If $s \neq p$ and $s \neq q$, then if $T \vdashg \proj{s}{\G}$ then $T \vdashg \residual{\comm{p}{\lambda}{q}}{ \proj{s}{\G} }$.

\end{itemize}

Thus we have that $\N' \vdashg \residual{ \comm{p}{\lambda}{q} }{ \boxplus_{k \in K'} \comm{r}{\mu_k}{s_k} ; \GH_k }$.
\comH{
 Here, various ways to conclude by observing that since for all $\ell \in K \setminus K'$, we have there is no $\M$ such that $\N \dgoesto{\comm{r}{\mu_\ell}{s_\ell}} \M$, then $\N \vdashg \boxplus_{k \in K'} \comm{r}{\mu_k}{s_k}; \GH_k$.
}

Thus we have that $\N' \vdashg \residual{\comm{p}{\lambda}{q}}{ \boxplus_{k \in K'} \comm{r}{\mu_k}{s_k}; \GH_k}$.
\end{proof}

Subject reduction should hold for almost all well-designed session type systems, hence there is little departure in the proof strategy: a global type is reconstructed after every transition.

The following lemma is where we appeal to justness.
\begin{lemma}{occurs app}
If $\N$ is guardedly well-typed and race-free,
and $p$ is not successfully terminated in $\N$, along every $\J$-path beginning with $\N$, there is some transition stemming from $p$.
%completed and some participant $p$ is enabled  contains a transition $t$ that is 
\end{lemma}
\begin{proof}
Consider a type $\G$ such that $\N \vdashg \G$
and a $J$-path of $\N$.
Also assume that $p$ has not successfully terminated.

\newcommand{\psize}[2]{ \left\| #1 \right\|_{#2} }

Define the maximum depth in the abstract syntax tree of $\G$ to a communication involving location $p$ to be $\psize{\G}{p}$. Observe this measure is well defined by guardedness, as long as $p$ is not successfuly terminated.
=======
>>>>>>> 38b2f901328a1664cea5bbd4296dcb4e98ad2e42
